# Supplementary material for: On Rollouts in Model-Based Reinforcement Learning
Source: arXiv:2501.16918 source file (2025-04-08)
Supplement: Supplementary file 1 [file appendix_writeup.tex]

\section{An Information Theoretic Perspective on Synthetic Rollouts in Model-Based Reinforcement Learning}
\subsection{Dynamics}
Let us consider dynamics of the form:
\begin{equation}
 \begin{aligned} 
 S_{t+1} &= \mu\left(S_t, A_t\right) + L\left(S_t, A_t\right) W_t \\ 
        &= f\left(S_t, A_t, W_t\right)
 \end{aligned}
 \end{equation}
where,
\[
    S_t, S_{t+1} \in \mathcal{S} \subseteq \mathbb{R}^{n_s}, \quad
    A_t \in \mathcal{A} \subseteq \mathbb{R}^{n_a}, \quad
    W_t \sim \mathcal\mathbb{N}(0, I_{n_s}).
\]
Here, $L(S_t, A_t)$ is the Cholesky decomposition of a covariance matrix $\Sigma$, given by:
\begin{equation}
    \Sigma\left(S_t, A_t\right)=L\left(S_t, A_t\right) L\left(S_t, A_t\right)^{\top}.
\end{equation}

In general, the following information theoretic relations hold\footnote{In the following, when we refer to entropies of continuous random variables (RVs), we use the quantized entropy given by $\mathbb{H}^{\Delta x}(X) = h(X) - \log_2 \Delta x$. Here $h(X)$ is the differential entropy of $X$, and $\mathbb{H}^{\Delta x}(X)$ is an approximation to the discrete entropy $\mathbb{H}(X)$ of the continuous RV $X \in \mathbb{R}$, with $\Delta x$ being a small discretization value ($10^{-6}$).}
\begin{equation}
\mathbb{H}\left(S_{t+1} \mid S_t=s_t, A_t=a_t\right)\geq0 
\label{ent_next_state_given_current}
\end{equation}
\begin{equation}
\mathbb{H}\left(S_{t+1} \mid S_t=s_t, A_t=a_t, W_t=w_t\right)=0
\label{ent_next_state_given_current_and_process}
\end{equation}

Equation \ref{ent_next_state_given_current} indicates that given some realization of the current state and action, there is a remaining entropy in the next state due to the process noise $W_t$. However, if we observe the value of $W_t$, then there is no remaining uncertainty, as shown in Equation \ref{ent_next_state_given_current_and_process}. Since $W_t$ is unobservable, some entropy always remains.
\subsection{Model}
We do not have access to the ground truth dynamics; instead, we rely on a model parametrized by $\theta$, such that:
\begin{equation}
    \begin{aligned}
    \hat{S}_{t+1, \theta} &= \hat{\mu}_\theta\left(S_t, A_t\right) + \hat{L}_\theta\left(S_t, A_t\right) W_t \\
    &= \hat{f}_\theta\left(S_t, A_t, W_t\right)
    \end{aligned}
\end{equation}

Here, $\theta$ is distributed according to some distribution $\mathbb{P}_\theta$, which we have access to or can approximate. We now consider the RV $\hat{S}_{t+1}$ obtained as:
\begin{equation}
\begin{aligned}
    \theta_t &\sim \mathbb{P}_\theta, \\
    \hat{S}_{t+1} &= \hat{\mu}_{\theta_t}(S_t, A_t) + \hat{L}_{\theta_t}(S_t, A_t) W_t \\
    &= \hat{f}_{\theta_t}(S_t, A_t, W_t)
\end{aligned}
\label{random_model_prediction}
\end{equation}

Now, we consider the problem of generating synthetic trajectories using our model. We denote by $\tilde S_{t}$ and $\tilde A_{t}$ the RVs representing the current imagined state and action respectively. Let us analyze how $S_{t+1}$ and $\hat{S}_{t+1}$ are obtained starting from $\tilde S_t = \tilde s_t$ and $\tilde A_t = \tilde a_t$. The RV $S_{t+1}$ is obtained as:
\begin{equation}
    \begin{aligned}
    W_t & \sim \mathcal{N}\left(0, I_{n_s}\right), \\
    S_{t+1} &= f\left(\tilde s_t, \tilde a_t, W_t\right)
    \end{aligned}
\end{equation}
The RV $\hat{S}_{t+1}$ is obtained as:
\begin{equation}
    \begin{aligned}
    \hat{W}_t & \sim \mathcal{N}\left(0, I_{n_s}\right), \\
    \theta_t & \sim \mathbb{P}_\theta, \\
    \hat{S}_{t+1}& =\hat{f}_{\theta_t}\left(\tilde s_t, \tilde a_t, \hat{W}_t\right)
    \end{aligned}
\end{equation}
where $W_t$, $\hat{W}_t$, and $\theta_t$ are mutually independent. We can see that $S_{t+1}$ and $\hat{S}_{t+1}$ are independent. Conventional rollouts proceed by using a realization of $\hat S_{t+1}$ to continue the next rollout step, that is, $\tilde S_{t+1} \leftarrow \hat S_{t+1}$. The RV $\hat{S}_{t+1}$ combines epistemic uncertainty from $\theta_t$ with aleatoric uncertainty from $\hat W_t$. We assume that each model has sufficient capacity to accurately represent the true dynamics. That is, model disagreements is attributed to epistemic uncertainty and not model inadequacy. Further, we assume that each model gives a consistent estimate of the true covariance $\Sigma$, that is\footnote{It might be useful to show that this holds in most cases somehow.},

\begin{equation}
    \left(\hat \Sigma_{\theta}\left(\tilde s_t, \tilde a_t\right) - \Sigma\left(\tilde s_t, \tilde a_t\right)\right) \geq 0 .
\end{equation}

In such a case, $\hat S_{t+1}$ will have a higher variance than $S_{t+1}$. This has serious implications when generating trajectories by autoregressively feeding in model prediction at the current step to generate the next transition. The predicted states' variance at each rollout step will grow faster than those corresponding to real trajectories. It will cause the model to hallucinate state transitions in physically infeasible parts of the state space when rolling out long trajectories. 
\subsection{Coupling and Information Loss}
To study how $\hat S_{t+1}$ deviates from $S_{t+1}$, we introduce a coupling:
\begin{equation}
    \hat{S}_{t+1}=S_{t+1}+b_{t+1}(\tilde s_t, \tilde a_t) + N_{t+1}
    \label{coupling}
\end{equation}

where $b_{t+1}(\tilde s_t, \tilde a_t)$ represents the model bias and $N_{t+1} \sim \mathcal{N}\left(0, \hat \Sigma^{\mathrm{epist}}(\tilde s_t, \tilde a_t)\right)$ is a random modeling noise. Further, we assume that given $\tilde S_t = \tilde s_t$ and $\tilde A_t = \tilde a_t$, $N_{t+1} \perp S_{t+1}$. Hence we consider $\hat{S}_{t+1}$ as a biased and noisy observation of $S_{t+1}$. This induces a joint distribution over $S_{t+1}$ and $\hat S_{t+1}$ such that its marginals coincide with the distributions of $S_{t+1}$ and $\hat S_{t+1}$ given $\tilde S_t = \tilde s_t$ and $\tilde A_t = \tilde a_t$. Now let us consider the task of inferring $S_{t+1}$ given an event $\hat{S}_{t+1}=\hat s_{t+1}$, that is the RV 
\begin{equation}
    S_{t+1} \mid \tilde S_t=s_t, \tilde A_t=a_t, \hat{S}_{t+1}=\hat{s}_{t+1}.
    \label{conditional}
\end{equation}

The following information-theoretic relations can be written,
\begin{equation}
    \mathbb{H}\left(S_{t+1} \mid \tilde S_t=\tilde s_t, \tilde A_t=\tilde a_t\right) \geq \mathbb{I}\left(S_{t+1}; \hat{S}_{t+1}=\hat{s}_{t+1} \mid \tilde S_t=s_t, \tilde A_t=a_t\right)
    \label{mutual_information_loss}
\end{equation}
\begin{equation}
    \mathbb{H}\left(S_{t+1} \mid \tilde S_t=s_t, \tilde A_t=a_t, \hat{S}_{t+1}=\hat{s}_{t+1}\right) \geq 0
    \label{entropy_buildup}
\end{equation}
Equations \ref{mutual_information_loss} and \ref{entropy_buildup} represent the loss in information that we incur when using a model prediction to infer the corresponding ground truth. Equality indicates a perfect model that has no epistemic uncertainty. To continue the rollout, we set
\begin{equation}
    \tilde{S}_{t+1} \leftarrow {S}_{t+1} \mid \tilde{S}_t = \tilde{s}_t, \tilde{A}_t = \tilde{a}_t, \hat{S}_{t+1} = \hat{s}_{t+1} 
    \label{next_step}
\end{equation}
and repeat the steps. Even though the relation in \eqref{coupling} is a valid coupling for each time-step $t$ given $\tilde S_t = \tilde s_t$ and $\tilde A_t = \tilde a_t$, we do not allow the random variable $\hat S_{t+1}$ to evolve independently since this will cause the variance to increase faster than realistic trajectories as we already discussed. Instead, by starting the next rollout step from a realization of the RV $\tilde S_{t+1}$ which is obtained from \eqref{next_step}, we prevent the variance growth which results from propagating $\hat S_{t+1}$ by basing each subsequent prediction based on a realistic state.

A single realization of the RV sequence $\tilde{S}_0, \tilde{A}_0, \hat{S}_1, \tilde{S}_1, \dots, \hat{S}_T$ represents a single rollout. The total information loss incurred during one such realization can be obtained as
\begin{equation}
    \begin{aligned}
& \mathbb{H}\left({S}_1, {S}_2 \ldots {S}_T \vert \tilde{S}_0=\tilde{s}_0, \tilde{A}_0=\tilde{a}_0, \hat{S}_1=\hat{s}_1 \ldots\hat{S}_T=\hat{s}_T\right) \\
& =\sum_{t=0}^{T-1} \mathbb{H}\left({S}_{t+1} \mid \tilde{S}_t=\tilde{s}_t, \tilde{A}_t=\tilde{a}_t, \hat{S}_{t+1}=\hat{s}_{t+1}\right)
\end{aligned}
\end{equation}

The above equation can be obtained by using the Markov property and causality. Hence, the total information lost is equal to the sum of the information lost at each rollout step.

However, in practice, we do not have access to the ground truth dynamics nor do we know the model bias or noise. In the next section, we discuss how we can approximate these in the context of probabilistic ensemble models.

\subsection{Rollout in Practice}
We now propose a practical rollout scheme using a probabilistic ensemble (PE) model that can approximately capture the loss of information depicted in \eqref{mutual_information_loss} and \eqref{entropy_buildup} which results from the coupling defined in \eqref{coupling}. We define the PE model as,
\begin{equation}
    \hat{f}_\theta = \left\{\hat{f}_{\theta_e}\right\}_{e=1}^E = \left\{\left(\hat{\mu}_{\theta_e}, \hat{L}_{\theta_e}\right)\right\}_{e=1}^E.
\end{equation}
Like before, we represent by $\tilde{S}_t$ and $\tilde{A}_t$ the RVs denoting the current state and action in our imagined trajectory. Given their realizations $\tilde{S}_t = \tilde{s}_t$ and $\tilde{A}_t = \tilde{a}_t$, we obtain the predictive distributions of each ensemble member as:
\begin{equation}
    \hat{S}_{t+1, \hat{\theta}_e} \sim \mathcal{N}\left(\hat{\mu}_{\theta_e}\left(\tilde{s}_t, \tilde{a}_t\right), \hat{\Sigma}_{\theta_e}\left(\tilde{s}_t, \tilde{a}_t\right)\right)
\end{equation}
where,
\begin{equation*}
    \hat{\Sigma}_{\theta_e}\left(\tilde{s}_t, \tilde{a}_t\right)=\hat{L}_{\theta_e}\left(\tilde{s}_t, \tilde{a}_t\right) \hat{L}_{\theta_e}\left(\tilde{s}_t, \tilde{a}_t\right)^{\top}
\end{equation*} 

A model prediction is then obtained as\footnote{Conventional rollouts proceed by setting $\tilde S_{t+1} \leftarrow \hat S_{t+1}$. We have already discussed how this is not suitable for long-horizon predictions. } 
\begin{equation}
\begin{split}
    e_t &\sim \mathcal U(1\dots E) \\
    \hat S_{t+1} &\sim \mathcal{N}\left(\hat{\mu}_{\theta_{e_t}}\left(\tilde{s}_t, \tilde{a}_t\right), \hat{\Sigma}_{\theta_{e_t}}\left(\tilde{s}_t, \tilde{a}_t\right)\right)
\end{split}
\end{equation}

First, we discuss how to obtain a proxy for ground truth dynamics. We can fuse the predictive distributions of each ensemble member to obtain a better estimate of ground truth predictive distribution, that is, 
\begin{equation}
    \mathcal{N}\left(\bar{\mu}_\Theta\left(\tilde{s}_t, \tilde{a}_t\right), \bar{\Sigma}_\Theta\left(\tilde{s}_t, \tilde{a}_t\right)\right) \approx \mathcal{N}\left(\mu\left(\tilde{s}_t, \tilde{a}_t\right), \Sigma\left(\tilde{s}_t, \tilde{a}_t\right)\right)
\end{equation}
where the bar notation represents fused estimate. Henceforth, we will use the RV 
\begin{equation}
    \bar{S}_{t+1}=\bar{\mu}_\Theta\left(\tilde{s}_t, \tilde{a}_t\right)+\bar{L}_\Theta\left(\tilde{s}_t, \tilde{a}_t\right) \bar{W}_t
\end{equation}
in the place of $S_{t+1}$.

We interpret the ensemble models as samples from the distribution $\mathbb P_{\theta}$. With this insight, we  
approximate  
\begin{equation}
    \hat{\Sigma}_{t+1}^{\text {epist }}\approx \frac{1}{E} \sum_{\theta=1}^E\left(\hat{\mu}_\theta-\bar{\mu}_\Theta\right)\left(\hat{\mu}_{\theta_e}-\bar{\mu}_\Theta\right)^\top.
\end{equation}

Finally, we consider the coupling

\begin{equation}
    \hat S_{t+1} = \bar S_{t+1} +  N_{t+1}
\end{equation}
with, $\bar S_{t+1} \perp  N_{t+1}$. This gives rise to the joint distribution of $\bar S_{t+1}$ and $\hat S_{t+1}$. Now, given a model prediction $\hat{S}_{t+1} = \hat{s}_{t+1}$, we can compute the distribution of $$\bar{S}_{t+1} \mid \tilde{S}_t = \tilde{s}_t, \tilde{A}_t = \tilde{a}_t, \hat{S}_{t+1} = \hat{s}_{t+1},$$ from which we can compute the conditional entropy
\begin{equation}
    \mathbb H(\bar{S}_{t+1} \mid \tilde{S}_t = \tilde{s}_t, \tilde{A}_t = \tilde{a}_t, \hat{S}_{t+1} = \hat{s}_{t+1}) 
\end{equation}
which we use to approximate the loss in information incurred in the current time step.

So far, we have not considered the bias $b_{t+1}$. Without further knowledge, it is not possible to approximate this. Our best option is to consider the model as being unbiased in the region where it has seen data. This is a reasonable assumption in our context because we assume that the true dynamics can be represented accurately where it has seen data. Hence we need to restrict the rollouts to the region where it has seen data. To do this in practice, in addition to considering accumulated information loss, we put a threshold on the per step information loss, such that, 
\begin{equation}
    \mathbb{H}\left(\bar{S}_{t+1} \mid \tilde{S}_t=\tilde{s}_t, \tilde{A}_t=\tilde{a}_t, \hat{S}_{t+1}=\hat{s}_{t+1}\right) < \lambda_{1}.
\end{equation}
The threshold $\lambda_{1}$ can be obtained by observing how the per step loss looks like within the model dataset\footnote{More information on this later}. This thresholding ensures that the information loss at each step is similar to how information loss looks when operating on seen data. Finally, given a trajectory realization, we can compute the information loss incurred through the trajectory as,

\begin{equation}
\begin{split}
    & \mathbb{H}\left({S}_1, {S}_2 \ldots {S}_T \vert \tilde{S}_0=\tilde{s}_0, \tilde{A}_0=\tilde{a}_0, \hat{S}_1=\hat{s}_1 \ldots\hat{S}_T=\hat{s}_T\right) \\
    & \approx \mathbb{H}\left(\bar {S}_1, \bar {S}_2 \ldots \bar {S}_T \vert \tilde{S}_0=\tilde{s}_0, \tilde{A}_0=\tilde{a}_0, \hat{S}_1=\hat{s}_1 \ldots\hat{S}_T=\hat{s}_T\right) \\
    & =\sum_{t=0}^{T-1} \mathbb{H}\left(\bar {S}_{t+1} \mid \tilde{S}_t=\tilde{s}_t, \tilde{A}_t=\tilde{a}_t, \hat{S}_{t+1}=\hat{s}_{t+1}\right)
\end{split}
\end{equation}

Finally, we can put a threshold on the accumulated information loss, that is,
\begin{equation}
    \sum_{t=0}^{T-1} \mathbb{H}\left(\bar {S}_{t+1} \mid \tilde{S}_t=\tilde{s}_t, \tilde{A}_t=\tilde{a}_t, \hat{S}_{t+1}=\hat{s}_{t+1}\right) < \lambda_{2}.
\end{equation}
Hence we no longer have to limit rollouts to a conservative maximum horizon, but rather control rollout lengths purely based on the proposed information loss.

 Therefore, we now have a way to:
\begin{enumerate}
    \item produce stable rollouts which reflect the process stochasticity more accurately,
    \item ensure rollouts lie within the region where it is sufficiently accurate,
    \item quantify accumulated information lost through the rollout process and control rollout lengths based on this.
\end{enumerate}
\newpage
